# Supplementary material for: X-World 1.6: Building Controllable Virtual Cities with World Models
Source: arXiv:2611.00596 source file (2026-11-21)
Supplement: Supplementary file 1 [file appendix.tex]

\section{Additional Details}
\label{sec:appendix_details}

Use the appendix for material that supports the paper but would interrupt the main narrative.
Typical appendix content includes extended implementation details, additional experiments, annotation instructions, proofs, extra qualitative examples, and dataset documentation.

\subsection{Reproducibility Checklist}

\begin{itemize}
    \item List software dependencies and versions.
    \item Specify hardware used for training and evaluation.
    \item Document random seeds and evaluation protocols.
    \item Provide links or instructions for code, models, and data when they are released.
\end{itemize}

\subsection{Additional Results}

Add supplementary tables, plots, and qualitative examples here.
